# Supplementary material for: CORRECT: Context- and Reference-Augmented Reasoning and Prompting for Fact-Checking
Source: arXiv:2502.09635 source file (2025-02-09)
Supplement: Supplementary file 1 [file additional_experiments.tex]

\section{Additional Experiment Results}
\label{sec:additional_experiments}

In the main paper, we mainly show the experiment results with Macro F1 score as evaluation metric. Here we further provide results with Micro F1 scores in Table \ref{table:fully_supervised_micro_f1} and Table \ref{table:5_shot_micro_f1} for fully supervised setting and 5-shot setting, respectively.

Overall, our model predicts veracity more accurately than baselines across all datasets, because of the advantage of incorporating both contextual and referential documents. By comparing to prompting-bases baselines that use natural language prompt, our model achieves better verification accuracy, since continuous and learnable prompt embeddings learned by our proposed evidence-conditioned prompt encoder are flexible and can better adapt to the dataset. Again, MultiVerS is slightly better than our model on SciFact dataset, mainly because most evidence sentences in this dataset are sufficient to verify the claims, and auxiliary referential documents do not bring much additional benefit.

\begin{table*}[t]
	\centering
	\caption{Verdict prediction results on \emph{fully supervised} setting with \emph{Micro F1} score. Results are in percentage.}
	%\vspace{-0.2cm}
	\resizebox{\textwidth}{!}{
		\begin{tabular}{c|cc|cc|cc|cc}
			\toprule
                \multirow{2}{*}{Model} & \multicolumn{2}{c|}{BearFact} & \multicolumn{2}{c|}{Check-COVID} & \multicolumn{2}{c|}{SciFact} & \multicolumn{2}{c}{FEVEROUS-S} \\
			\cline{2-9}
			{} & Gold & Retrieved & Gold & Retrieved & Gold & Retrieved & Gold & Retrieved \\
			\hline
                KGAT & 69.42$ \pm $0.87 & 57.36$ \pm $0.52 & 72.05$ \pm $1.58 & 76.47$ \pm $0.65 & 74.44$ \pm $0.96 & 62.33$ \pm $0.88 & 86.21$ \pm $0.28 & 67.99$ \pm $0.78 \\
                HESM & 63.68$ \pm $1.39 & 58.62$ \pm $0.32 & 63.47$ \pm $0.25 & 71.90$ \pm $1.85 & 72.44$ \pm $0.77 & 53.36$ \pm $2.33 & 83.30$ \pm $0.75 & 68.36$ \pm $0.86 \\
                Transformer-XH & 61.26$ \pm $0.72 & 56.55$ \pm $1.50 & 68.56$ \pm $0.87 & 76.91$ \pm $1.51 & 75.89$ \pm $0.51 & 58.67$ \pm $1.53 & 85.61$ \pm $0.80 & 69.78$ \pm $0.41 \\
                Transformer-XH++ & 64.02$ \pm $1.44 & 58.39$ \pm $1.11 & 70.60$ \pm $0.67 & 78.65$ \pm $0.38 & 77.78$ \pm $0.69 & 60.56$ \pm $1.83 & 85.52$ \pm $0.39 & 70.37$ \pm $0.77 \\
                MultiVerS & 62.93$ \pm $1.17 & 50.69$ \pm $1.46 & 66.65$ \pm $1.71 & 70.70$ \pm $1.73 & 83.68$ \pm $1.40 & \textbf{66.77}$ \pm $\textbf{0.14} & 83.57$ \pm $1.54 & 67.66$ \pm $1.65 \\
                CausalWalk & 69.31$ \pm $1.69 & 60.00$ \pm $0.69 & 71.86$ \pm $1.54 & 71.68$ \pm $2.48 & 77.34$ \pm $2.30 & 59.00$ \pm $1.20 & 86.42$ \pm $0.92 & 71.51$ \pm $1.66 \\
                \hline
                GPT2-PPL & 40.00$ \pm $2.43 & 39.49$ \pm $0.73 & 32.75$ \pm $0.62 & 32.54$ \pm $0.93 & 31.50$ \pm $0.71 & 31.24$ \pm $1.56 & 54.33$ \pm $0.06 & 54.23$ \pm $0.01 \\
                ProToCo & 56.03$ \pm $0.24 & 35.57$ \pm $2.35 & 37.12$ \pm $1.10 & 32.75$ \pm $2.31 & 60.00$ \pm $1.53 & 31.17$ \pm $0.71 & 54.21$ \pm $0.67 & 44.71$ \pm $1.95 \\
                ProgramFC & 62.00$ \pm $2.83 & 54.63$ \pm $3.66 & 65.50$ \pm $2.12 & 72.36$ \pm $1.85 & 65.40$ \pm $3.78 & 59.76$ \pm $3.54 & 86.48$ \pm $0.33 & 69.50$ \pm $2.12 \\
                \hline
                P-Tuning v2 & 70.69$ \pm $0.49 & 60.34$ \pm $0.15 & 72.93$ \pm $1.85 & 77.32$ \pm $1.96 & 80.34$ \pm $0.94 & 57.44$ \pm $1.83 & 87.16$ \pm $0.33 & 70.56$ \pm $0.54 \\
                \hline
                JustiLM & 62.41$ \pm $1.25 & 48.49$ \pm $2.21 & 59.71$ \pm $2.56 & 61.71$ \pm $2.05 & 72.20$ \pm $1.85 & 54.74$ \pm $0.82 & 81.60$ \pm $0.33 & 68.38$ \pm $1.45 \\
                \hline
                CORRECT & \textbf{74.60}$ \pm $\textbf{1.11} & \textbf{61.84}$ \pm $\textbf{0.11} & \textbf{75.33}$ \pm $\textbf{0.93} & \textbf{80.83}$ \pm $\textbf{0.76} & \textbf{85.17}$ \pm $\textbf{0.71} & 63.50$ \pm $1.17 & \textbf{88.51}$ \pm $\textbf{0.19} & \textbf{75.35}$ \pm $\textbf{0.28} \\
			\bottomrule
		\end{tabular}
	}
	%\vspace{-0.3cm}
	\label{table:fully_supervised_micro_f1}
\end{table*}

\begin{table*}[t]
	\centering
	\caption{Verdict prediction results on \emph{5-shot} setting with \emph{Micro F1} score. Results are in percentage.}
	%\vspace{-0.2cm}
	\resizebox{\textwidth}{!}{
		\begin{tabular}{c|cc|cc|cc|cc}
			\toprule
                \multirow{2}{*}{Model} & \multicolumn{2}{c|}{BearFact} & \multicolumn{2}{c|}{Check-COVID} & \multicolumn{2}{c|}{SciFact} & \multicolumn{2}{c}{FEVEROUS-S} \\
			\cline{2-9}
			{} & Gold & Retrieved & Gold & Retrieved & Gold & Retrieved & Gold & Retrieved \\
			\hline
                KGAT & 44.66$ \pm $0.25 & 36.78$ \pm $3.86 & 37.55$ \pm $2.86 & 50.98$ \pm $1.13 & 42.22$ \pm $3.06 & 36.78$ \pm $3.52 & 51.13$ \pm $1.55 & 51.66$ \pm $1.38 \\
                HESM & 48.85$ \pm $2.42 & 28.97$ \pm $3.26 & 36.68$ \pm $5.15 & 50.11$ \pm $3.22 & 39.56$ \pm $2.45 & 35.89$ \pm $4.67 & 56.33$ \pm $0.91 & 53.68$ \pm $0.37 \\
                Transformer-XH & 32.53$ \pm $3.13 & 40.80$ \pm $3.32 & 41.67$ \pm $2.19 & 51.63$ \pm $1.16 & 48.89$ \pm $2.84 & 35.11$ \pm $1.95 & 52.94$ \pm $2.65 & 51.56$ \pm $0.73 \\
                Transformer-XH++ & 37.93$ \pm $4.10 & 35.06$ \pm $3.66 & 41.40$ \pm $1.78 & 52.41$ \pm $1.22 & 50.00$ \pm $0.85 & 36.67$ \pm $1.65 & 59.97$ \pm $1.50 & 53.23$ \pm $1.19 \\
                MultiVerS & 40.86$ \pm $0.74 & 39.49$ \pm $1.70 & 41.01$ \pm $1.29 & 49.82$ \pm $1.56 & \textbf{54.99}$ \pm $\textbf{1.90} & 43.33$ \pm $1.74 & 51.39$ \pm $1.33 & 51.84$ \pm $1.54 \\
                CausalWalk & 45.52$ \pm $3.47 & 41.38$ \pm $3.24 & 37.70$ \pm $4.59 & 43.79$ \pm $3.25 & 44.02$ \pm $2.70 & 41.78$ \pm $2.71 & 60.60$ \pm $1.98 & 55.20$ \pm $4.18 \\
                \hline
                GPT2-PPL & 36.38$ \pm $4.14 & 40.69$ \pm $0.49 & 33.19$ \pm $0.67 & 34.62$ \pm $0.72 & 29.44$ \pm $2.50 & 29.00$ \pm $1.46 & 53.02$ \pm $1.11 & 53.11$ \pm $1.12 \\
                ProToCo & 51.03$ \pm $2.44 & 33.80$ \pm $2.44 & 41.05$ \pm $2.47 & 34.50$ \pm $2.31 & 51.55$ \pm $2.27 & 36.78$ \pm $1.35 & 54.72$ \pm $1.32 & 42.45$ \pm $2.73 \\
                ProgramFC & 38.45$ \pm $2.19 & 38.28$ \pm $0.49 & 37.55$ \pm $0.38 & 50.00$ \pm $1.08 & 49.93$ \pm $0.36 & 36.17$ \pm $1.25 & 52.94$ \pm $2.67 & 51.94$ \pm $0.25 \\
                \hline
                P-Tuning v2 & 48.70$ \pm $1.95 & 41.90$ \pm $3.10 & 41.05$ \pm $3.88 & 52.07$ \pm $3.09 & 45.78$ \pm $1.07 & 37.67$ \pm $1.85 & 58.02$ \pm $1.68 & 52.06$ \pm $0.76 \\
                \hline
                JustiLM & 42.70$ \pm $1.64 & 37.72$ \pm $5.08 & 40.82$ \pm $2.20 & 46.73$ \pm $1.53 & 47.41$ \pm $1.07 & 33.00$ \pm $1.58 & 52.54$ \pm $1.71 & 49.38$ \pm $1.60 \\
                \hline
                CORRECT & \textbf{51.72}$ \pm $\textbf{1.04} & \textbf{42.76}$ \pm $\textbf{0.73} & \textbf{43.37}$ \pm $\textbf{1.82} & \textbf{54.46}$ \pm $\textbf{0.76} & 53.00$ \pm $1.30 & \textbf{44.36}$ \pm $\textbf{0.84} & \textbf{63.33}$ \pm $\textbf{0.91} & \textbf{57.14}$ \pm $\textbf{0.82} \\
			\bottomrule
		\end{tabular}
	}
	%\vspace{-0.3cm}
	\label{table:5_shot_micro_f1}
\end{table*}
